# Supplementary material for: Weak ergodicity breaking captured from short-time dynamcis and graph theory
Source: arXiv:2605.00094 source file (2026-11-11)
Supplement: Supplementary file 1 [file supplemental.tex]

\documentclass[aps,prb,reprint,superscriptaddress,longbibliographw,showpacs,nobibnotes,nofootinbib,onecolumn]{revtex4-2}

\usepackage[utf8]{inputenc}
\usepackage[T1]{fontenc}
\usepackage[]{lmodern}
\usepackage[]{microtype}
\usepackage{physics}
\usepackage{mathtools}

\usepackage[english]{babel}
\usepackage[]{csquotes}

\makeatletter
\adddialect\l@en\l@english
\makeatother

\usepackage[]{amsmath}
\usepackage[]{amssymb,bbold}
\usepackage[mathscr]{euscript}

\usepackage{siunitx}
\sisetup{range-phrase=\,\textup{--}}

\usepackage[]{graphicx}
\usepackage[]{tabularx}
\usepackage[figurename=Figure]{caption}
\usepackage[]{subcaption}

\usepackage{xcolor}

\usepackage{ragged2e}
\DeclareCaptionJustification{plain}{\justifying}
\captionsetup{
	justification = plain,
	singlelinecheck = false
}

\usepackage[]{hyperref}
\hypersetup{
    colorlinks=true,
    urlcolor=blue,
    citecolor=blue,
    linkcolor=blue
}
\usepackage[capitalize]{cleveref}
\crefname{table}{Tab.}{Tab.}

\renewcommand{\var}{\mathop{\mathrm{Var}}\nolimits}

\DeclareMathOperator{\GEC}{\mathsf{GEC}}

\newcommand{\qmoperator}[1]{\ensuremath{\hat{#1}}}
\DeclareMathOperator{\hc}{h.c.}

\newcommand{\ie}{{ i.e.},\ }

\usepackage{comment}

%\newcommand{\hgm}[1]{{\color{blue}#1}}
%\newcommand{\rsw}[1]{{\color{red}#1}}
%\newcommand{\mcb}[1]{{\color{green}#1}}
%\newcommand{\fhm}[1]{{\color{brown}#1}}
%\newcommand{\vanishchanges}[1]{{\color{blue}#1}}
% Uncomment these commands to get rid of highlights and explanation texts.
%\renewcommand{\changes}[1]{#1}

\begin{document}
\setcounter{figure}{0}
\setcounter{equation}{0}
\setcounter{table}{0}
\setcounter{section}{0}

\renewcommand{\thetable}{S\arabic{table}}
\renewcommand{\thefigure}{S\arabic{figure}}
\renewcommand{\theequation}{S\arabic{equation}}
\renewcommand{\thepage}{S\arabic{page}}

\renewcommand{\thesection}{S\arabic{section}}

\title{Supplementary material to \enquote{Graph-theory measures capture weak ergodicity breaking on large quantum systems}}

\author{Heiko Georg Menzler}
\affiliation{Institut für Theoretische Physik, Georg-August-Universität Göttingen, D-37077 Göttingen, Germany}

\author{Rafał Świętek}
\affiliation{Institut für Theoretische Physik, Georg-August-Universität Göttingen, D-37077 Göttingen, Germany}

\author{Mari Carmen Ba\~nuls}
\affiliation{Max-Planck-Institut für Quantenoptik, D-85748 Garching, Germany}
\affiliation{Munich Center for Quantum Science and Technology (MCQST), Schellingstrasse 4, D-80799 München, Germany}

\author{Fabian Heidrich-Meisner}
\affiliation{Institut für Theoretische Physik, Georg-August-Universität Göttingen, D-37077 Göttingen, Germany}

\maketitle
\section{\texorpdfstring{Details on the $\GEC$ measure}{Details on the GEC measure}}\label{sm:sec:gec}
Given a traceless Hamiltonian $\qmoperator H \to \qmoperator H-\Tr(\qmoperator H)/D$, we define the $\GEC$ for a basis state $\ket{i}$ as
\begin{align}\label{sm:eq:gec:def0}
    \GEC(\ket{i}) = \frac{\Tr(\qmoperator H^2) - \Tr([\qmoperator H\setminus \ket{i}]^2)}{\Tr(\qmoperator H^2)/D}\,,
\end{align}
where $\qmoperator H\setminus \ket{i} \coloneq (\mathbb{1} - \ketbra{i}{i})\qmoperator H(\mathbb{1}-\ketbra{i}{i})$ projects the basis state $\ket{i}$ out of the Hilbert space, while $D$ is the Hilbert space dimension.
In this work, we normalize the $\GEC$ by a factor of $D$ in contrast to~\cite{Menzler2025}.
We can rewrite the definition of the $\GEC$ in \cref{sm:eq:gec:def} by employing the matrix elements of the Hamiltonian as
\begin{equation}\label{sm:eq:gec:def}
    \GEC(\ket{i}) = \frac{2(\qmoperator H^2)_{ii}-H_{ii}^2}{\frac{1}{D}\Tr{\qmoperator H^2}}\,,
\end{equation}
using the short form $H_{ij} = \mel{i}{\qmoperator H}{j}$ here and in the remainder of the text.

In this work, we are interested in finding the moments of the $\GEC$ distribution, where we consider the average over basis states $\ket{i}$ and, for the RPM and QSM, an additional average over Hamiltonian realizations.
Within each ensemble realization we define a set of random variables $a_i$ [for instance, $a_i\equiv \GEC(\ket{i})$] for each basis state $\ket{i}$ and define the average $\mathbb{E}[a] = \overline{(1/D)\sum_{i=1}^Da_i}$, where $\overline{\vphantom{\sum}\ldots}$ denotes an average over Hamiltonian realizations, for example $\mathbb{E}[\GEC]=\overline{(1/D)\sum_{i=1}^D\GEC(\ket{i})}$.
Note that since the denominator in \cref{sm:eq:gec:def} is independent of the state $\ket{i}$, the average over basis states affects only the numerator of the $\GEC$.
Additionally, when an average over different Hamiltonian realizations is required (RPM and QSM cases), our strategy is to perform it independently for the numerator and the denominator.
We denote the numerator by $x_i\equiv 2(\qmoperator H^2)_{ii}-H_{ii}^2$ and define the average strategy for the moments of the $\GEC$ as
\begin{equation}\label{sm:eq:gec:approx:moments}
    \mathbb{E}[\GEC] \approx \frac{1}{D\overline{\sigma^2}}\overline{\sum_{i=1}^Dx_i}
    \qquad\text{and}\qquad
    \var[\GEC] \approx \frac{1}{\qty(D\overline{\sigma^2})^2}\overline{\qty(\sum_{i=1}^Dx_i^2
    -
    \qty[\sum_{i=1}^Dx_i]^2)}
    \,.
\end{equation}
Here, we again define the width of the spectrum $\sigma^2=\frac{1}{D}\Tr{\qmoperator H^2}$.
We expect this approximation to become exact when $L \to \infty$, however, for finite system sizes, the leading corrections cannot always be obtained accurately,
which is tested and discussed in \cref{sm:sec:approx:validity}.

\section{\texorpdfstring{Derivation of the $\GEC$ for the RPM}{Derivation of the GEC for the RPM}}
Let us first start with the moments of the $\GEC$ for the RPM, which is defined by the Hamiltonian
\begin{equation}\label{sm:eq:rp}
    \qmoperator H_\mathrm{RP} = \qmoperator H_0+D^{-\gamma/2} \qmoperator M\,,
\end{equation}
with $\qmoperator H_\mathrm{GOE}$ being a $D\times D$ GOE matrix.
For completeness, we also write down the square of the Hamiltonian
\begin{equation}\label{sm:eq:rp:squared}
    \qmoperator H_\mathrm{RP}^2 = 
    \qmoperator H_0^2
    +
    D^{-\gamma} \qmoperator M^2
    +
    D^{-\gamma/2} (\qmoperator H_0\qmoperator M + \qmoperator M\qmoperator H_0)
    \,.
\end{equation}
The diagonal matrix $\qmoperator H_0$ has entries $\epsilon_i$ that are distributed according to some probability distribution $P(\epsilon)$.
We choose $P(\epsilon)$ to be normal distributed with unit variance in Sec.~\ref{sm:sec:approx:validity} and in the main text.
The mean of the diagonal elements vanishes, i.e., $\mathbb{E}[\epsilon]=0$, since we consider traceless Hamiltonians.
The elements of $\qmoperator M$ are distributed according to a Gaussian distribution with mean $0$ and variance $1$ for off-diagonal elements and $2$ for the diagonal matrix elements.

The parameter $\gamma$ controls the strength of off-diagonal couplings and drives the system across two critical points that separate distinct dynamical regimes~\cite{Rosenzweig1960,Altland1997,Kravtsov2015,Facoetti2016,Soosten2019,DeTomasi2019,Skvortsov2022,Barney2023,Venturelli2023}. 
For $\gamma < 1$, the model reproduces the spectral statistics of the GOE. 
In contrast, for $\gamma > 2$, the system enters a localized regime~\cite{Soosten2019}, where off-diagonal terms become negligible and the spectrum follows Poisson statistics. 
The intermediate regime, $1 < \gamma < 2$, is particularly rich, exhibiting nontrivial behavior in both eigenstate properties~\cite{Kravtsov2015,Bogomolny2018,DeTomasi2019,Soosten2019,DeTomasi2020} and spectral statistics~\cite{DeTomasi2019,Skvortsov2022,Barney2023,Venturelli2023,Buijsman2024}.

In this intermediate regime of the RPM, eigenfunctions acquire a fractal structure. This regime is sometimes referred to as nonergodic extended phases~\cite{Kravtsov2015,Bogomolny2018}.
We will refer to the intermediate regime as the fractal regime in the following.
These states are extended but occupy a vanishing fraction of the Hilbert space in the thermodynamic limit~\cite{DeTomasi2020}. 
This phase is associated with a breakdown of conventional random-matrix theory predictions, while still displaying universal features in the long-time dynamics of observables.
Specifically, the average gap ratio remains GOE-like, while the eigenstate fractal dimension yields a nonergodic value.
The fractal nature of eigenstates can be quantified by the generalized inverse participation ratio.
In particular, the model exhibits a well-defined fractal dimension $d_q = 2 - \gamma$ for $q > 1/2$~\cite{Kravtsov2015,Truong2016,Bogomolny2018}.

From the point of view of observable dynamics, the fractal phase in the RPM at $1<\gamma<2$ has been also identified as a fading-ergodicity regime.
Particularly, when the RPM is expressed in a many-body basis of $L$ spin-$1/2$ degrees of freedom, the matrix elements of  observables in the Hamiltonian eigenbasis do not obey ETH.
Additionally, quantum-quench dynamics show relaxation towards a thermal state in exponentially large timescales, which are shorter than the Heisenberg time of the system, see Ref.~\cite{Swietek2025a} for details.

It was shown that the width of the RPM is~\cite{Venturelli2023}
\begin{equation}\label{sm:eq:rp2}
    \frac{1}{D}\Tr{\qmoperator H^2_\mathrm{RP}} = \mathbb{E}[\epsilon^2]+D^{1-\gamma}+D^{-\gamma}\,.
\end{equation}
Following Eqs.~\eqref{sm:eq:rp} and~\eqref{sm:eq:rp:squared}, we can write down the different terms entering the $\GEC$
\begin{align}
    H_{ii}^2 &= \epsilon_i^2 + D^{-\gamma}M_{ii}^2+2D^{-\gamma/2}\epsilon_{i}M_{ii}\,,\\
    \qty(\qmoperator H^2)_{ii} &= \epsilon_i^2 + D^{-\gamma}\sum_jM_{ij}^2+2D^{-\gamma/2}\epsilon_{i}M_{ii}\,,
\end{align}
which leads to
\begin{equation}\label{sm:eq:rp:x_i}
    x_i = \epsilon_i^2 
    + 2D^{-\gamma}\sum_{j}M_{ij}^2
    + 2D^{-\gamma/2}\epsilon_{i}M_{ii}
    - D^{-\gamma}M_{ii}^2\,.
\end{equation}
Let us note that the following calculations for the RPM do not depend on the particular form of the basis states $\ket{i}$ as we only take into account the moments of the elements of the matrices $\hat{H}_0$ and $\hat{M}$.

\subsection{\texorpdfstring{Mean of the $\GEC$}{Mean of the GEC}}
The random variables $\epsilon_i$ and $M_{ij}$ are drawn independently from a random distribution, thus their averages factorize $\overline{\epsilon_i^kM_{ij}^m} = \overline{\epsilon_i^k}\overline{M_{ij}^m}$.
Therefore, any term containing odd moments of $M_{ij}$ vanishes, as the distribution of $M_{ij}$ is Gaussian.
The remaining terms are $\overline{M_{ii}^2}=2$ and $\frac{1}{D}\sum_{ij}\overline{M_{ij}^2}=\sum_{j\neq i}\overline{M_{ij}^2}+\frac{1}{D}\sum_i\overline{M_{ii}^2}=D-1+2 = D+1$, hence we obtain the average
\begin{equation}\label{sm:eq:rp:x_i:av}
    \mathbb{E}[x] = \mathbb{E}[\epsilon^2] + 2D^{1-\gamma}\,,
\end{equation}
Finally, the $\GEC$ can be expressed as
\begin{equation}\label{sm:eq:rp:GEC:mean}
    \mathbb{E}[\GEC] 
    =
    \frac{\mathbb{E}[\epsilon^2] + 2D^{1-\gamma}}{\mathbb{E}[\epsilon^2]+D^{1-\gamma}+D^{-\gamma}}
    = 
    1 + \frac{D^{1-\gamma} - D^{-\gamma}}{\mathbb{E}[\epsilon^2]+D^{1-\gamma}+D^{-\gamma}}\,.
\end{equation}
Remarkably, the transition from the ergodic into the fractal phase at $\gamma=1$ is already captured in the mean of the $\GEC$.
This expression obeys the following limiting cases: In the ergodic regime ($\gamma<1$), the mean of the $\GEC$ follows the expression
\begin{equation}\label{sm:eq:rp:GEC:mean:ergodic}
    \mathbb{E}[\GEC]_{\gamma<1}= 2 - \frac{\mathbb{E}[\epsilon^2]}{D^{1-\gamma}}+g_1(\gamma,D)\,,
\end{equation}
where the subleading correction captured by $g_1(\gamma, D)$ changes from $g_1(\gamma,D)=O(D^{-1})$ at $\gamma<1/2$ to $g_1(\gamma, D)=O(D^{2-2\gamma})$ for $1/2<\gamma<1$.
In contrast, for $\gamma > 1$ we find
\begin{equation}\label{sm:eq:rp:GEC:mean:fractal}
    \mathbb{E}[\GEC]_{\gamma>1} = 1 + \frac{1}{\mathbb{E}[\epsilon^2]D^{\gamma-1}}+g_2(\gamma,D)\,.
\end{equation}
We collect the subleading corrections to the mean of the $\GEC$ in the function $g_2(\gamma,D)$.
Remarkably, at the ergodicity-breaking transition for $\gamma=2$, the subleading correction changes from $g_2(\gamma\leq2,D)=O(D^{2-2\gamma})$ to $g_2(\gamma>2,D)=O(D^{-\gamma})$.
At the wEBT, when entering the fractal phase at $\gamma=1$, we identify the leading terms as
\begin{equation}\label{sm:eq:rp:GEC:mean:transition}
    \mathbb{E}[\GEC]_{\gamma=1} = \frac{\mathbb{E}[\epsilon^2]+2}{\mathbb{E}[\epsilon^2]+1} - \frac{\mathbb{E}[\epsilon^2]+2}{(1+\mathbb{E}[\epsilon^2])^2}\frac{1}{D}+O(D^{-2})\,.
\end{equation}
Therefore, for Gaussian-distributed elements with unit variance of the diagonal matrix $\hat{H}_0$, we find $\mathbb{E}[\GEC]_{\gamma=1}=\frac{3}{2}$ at the wEBT.

\subsection{\texorpdfstring{Variance of the $\GEC$}{Variance of the GEC}}
Next, we compute the variance of the $\GEC$, \ie the variance of $x_i$ in \cref{sm:eq:rp:x_i}.
We write the square of $x_i$ as $x_i^2=4(\qmoperator H^2)_{ii}^2+H_{ii}^4-4(\qmoperator H^2)_{ii}H_{ii}^2$.

Let us start with the first term of the form
    \begin{equation}\label{sm:eq:rp:Hii4}
        \begin{split}
        \frac{1}{D}\sum_i\overline{H_{ii}^4}
        &=
        \frac{1}{D}\sum_i\overline{\qty(\epsilon_i^2 + D^{-\gamma}M_{ii}^2+2D^{-\gamma/2}\epsilon_{i}M_{ii})^2}\\
        &=
        \mathbb{E}[\epsilon^4]
        +D^{-2\gamma}\frac{1}{D}\sum_i\overline{M_{ii}^4}
        +4D^{-\gamma}\mathbb{E}[\epsilon^2]\frac{1}{D}\sum_i\overline{M_{ii}^2}\\
        &\qquad
        +2D^{-\gamma}\mathbb{E}[\epsilon^2]\frac{1}{D}\sum_i\overline{M_{ii}^2}
        +4D^{-\gamma/2}\mathbb{E}[\epsilon^3]\frac{1}{D}\sum_i\overline{M_{ii}}
        +4D^{-3\gamma/2}\mathbb{E}[\epsilon]\frac{1}{D}\sum_i\overline{M_{ii}^3}\\
        &=
        \mathbb{E}[\epsilon^4] + 12D^{-2\gamma} + 12D^{-\gamma}\mathbb{E}[\epsilon^2]\,.
        \end{split}
    \end{equation}
    In the last equality, we use the fact that all odd moments of a Gaussian random variable vanish, $\mathbb{E}[M_{ii}^3]=\mathbb{E}[M_{ii}]=0$, and that the fourth moment can be found as $\mathbb{E}[M_{ii}^4]=3\mathbb{E}[M_{ii}^2]^2=12$.
    The next term can be calculated by expanding the sums into diagonal and off-diagonal terms with
    \begin{equation}
        \begin{split}
        \frac{1}{D}\sum_i\overline{(\qmoperator H^2)_{ii}^2}
        &=
        \mathbb{E}[\epsilon^4]
        +D^{-2\gamma}\frac{1}{D}\sum_{i,j,j'}\overline{M_{ij}^2M_{ij'}^2}
        +4D^{-\gamma}\mathbb{E}[\epsilon^2]\frac{1}{D}\sum_i\overline{M_{ii}^2}\\
        &\qquad
        +2D^{-\gamma}\mathbb{E}[\epsilon^2]\frac{1}{D}\sum_{i,j}\overline{M_{ij}^2}
        +4D^{-\gamma/2}\mathbb{E}[\epsilon^3]\frac{1}{D}\sum_i\overline{M_{ii}}
        +4D^{-3\gamma/2}\mathbb{E}[\epsilon]\frac{1}{D}\sum_{i,j}\overline{M_{ii}M_{ij}^2}\\
        &=
        \mathbb{E}[\epsilon^4]
        +D^{-2\gamma}\frac{1}{D}\sum_{i,j,j'}\overline{M_{ij}^2M_{ij'}^2}
        +8D^{-\gamma}\mathbb{E}[\epsilon^2]
        +2D^{-\gamma}(D+1)\mathbb{E}[\epsilon^2]\,,
        \end{split}
    \end{equation}
    where again, all odd moments of $M_{ij}$ vanish and we use the previous result $\sum_j\mathbb{E}[M_{ij}^2]=D+1$.
    By decomposing the remaining sum into diagonal and off-diagonal terms (removing the terms for which $i=j$ and $i=j'$ from the sums), we find
    \begin{equation}\label{sm:eq:rp:M2ii2}
        \begin{split}
        \frac{1}{D}\sum_{i,j,j'}\overline{M_{ij}^2M_{ij'}^2}
        &= 
        \frac{1}{D}\sum_{i,j'}\overline{M_{ii}^2M_{ij'}^2}
        +\frac{1}{D}\sum_{j\neq i,j'}\overline{M_{ij}^2M_{ij'}^2}\\
        &=
        \frac{1}{D}\sum_i\overline{M_{ii}^4}
        +\frac{1}{D}\sum_{j'\neq i}\overline{M_{ii}^2}\,\overline{M_{ij'}^2}
        +\frac{1}{D}\sum_{j\neq i}\overline{M_{ij}^2}\,\overline{M_{ii}^2}
        +\frac{1}{D}\sum_{j\neq i,j'\neq i}\overline{M_{ij}^2M_{ij'}^2}\\
        &=12+2(D-1)+2(D-1)
        +\frac{1}{D}\sum_{j\neq i}\overline{M_{ij}^4}
        +\frac{1}{D}\sum_{j\neq i,j'\neq i,j\neq j'}\overline{M_{ij}^2}\,\overline{M_{ij'}^2}\\
        &=8+4D+3(D-1)+(D-1)(D-2) = D^2+4D+7\,.
        \end{split}
    \end{equation}
    This leads to the result
    \begin{equation}\label{sm:eq:rp:H2ii2}
        \frac{1}{D}\sum_i\overline{(\qmoperator H^2)_{ii}^2} = \mathbb{E}[\epsilon^4]+D^{2-2\gamma}+4D^{1-2\gamma}+7D^{-2\gamma}+10D^{-\gamma}\mathbb{E}[\epsilon^2]+2D^{1-\gamma}\mathbb{E}[\epsilon^2]\,.
    \end{equation}
    The last term requires slightly more care, but following similar steps we obtain
    \begin{equation}\label{sm:eq:rp:H2iiHii2}
        \begin{split}
        \frac{1}{D}\sum_i{(\qmoperator H^2)_{ii}H_{ii}^2}
        &=
        \mathbb{E}[\epsilon^4]
        +D^{-\gamma}\mathbb{E}[\epsilon^2]\frac{1}{D}\sum_i{M_{ii}^2}
        +2D^{-\gamma/2}\mathbb{E}[\epsilon^3]\frac{1}{D}\sum_i{M_{ii}}\\
        &\qquad
        +D^{-\gamma}\mathbb{E}[\epsilon^2]\frac{1}{D}\sum_{i,j}\overline{M_{ij}^2}
        +D^{-\gamma}\frac{1}{D}\sum_{i,j}\overline{M_{ii}^2M_{ij}^2}
        +2D^{-3\gamma/2}\mathbb{E}[\epsilon]\frac{1}{D}\sum_i{M_{ii}}\frac{1}{D}\sum_{i,j}\overline{M_{ij}^2}\\
        &\qquad
        +2D^{-\gamma/2}\mathbb{E}[\epsilon^3]\frac{1}{D}\sum_i\overline{M_{ii}}
        +2D^{-3\gamma/2}\mathbb{E}[\epsilon]\frac{1}{D}\sum_i\overline{M_{ii}^3}
        +4D^{-\gamma}\mathbb{E}[\epsilon^2]\frac{1}{D}\sum_i\overline{M_{ii}^2}\\
        &=
        \mathbb{E}[\epsilon^4]+11D^{-\gamma}\mathbb{E}[\epsilon^2]+D^{1-\gamma}\mathbb{E}[\epsilon^2]+2D^{1-2\gamma}+10D^{-2\gamma}\,,
        \end{split}
    \end{equation}
    where in the last equality we use
    \begin{equation}\label{sm:eq:rp:M2iiMii2}
        \frac{1}{D}\sum_{i,j}\overline{M_{ii}^2M_{ij}^2} 
        = 
        \frac{1}{D}\sum_{i}\overline{M_{ii}^4}
        +
        \frac{1}{D}\sum_{j\neq i}\overline{M_{ii}^2}\,\overline{M_{ij}^2}=2D+10\,.
    \end{equation}

Collecting Eqs.~\eqref{sm:eq:rp:Hii4}--\eqref{sm:eq:rp:H2iiHii2} yields the expression for the second moment of $x_i$
\begin{equation}\label{sm:eq:rp:x_i2}
    \mathbb{E}[x^2]
    =
    \mathbb{E}[\epsilon^4]+8D^{-\gamma}\mathbb{E}[\epsilon^2]+4D^{1-\gamma}\mathbb{E}[\epsilon^2]
    +4D^{2-2\gamma}+8D^{1-2\gamma}\,.
\end{equation}
Together with the square of the second moment [defined in \cref{sm:eq:rp:x_i:av}], we find
\begin{equation}\label{sm:eq:rp:x_i:av2}
    \mathbb{E}[x]^2 = \mathbb{E}[\epsilon^2]^2 + 4D^{2-2\gamma} + 4\mathbb{E}[\epsilon^2]D^{1-\gamma}\,.
\end{equation}
The final expression for the variance of the $\GEC$ in the RPM is
\begin{equation}\label{sm:eq:rp:GEC:var}
    \var[\GEC]=\mathbb{E}[\GEC^2]-\mathbb{E}[\GEC]^2
    =
    \frac{\mathbb{E}[\epsilon^4]-\mathbb{E}[\epsilon^2]^2 + 8D^{-\gamma}\mathbb{E}[\epsilon^2]+8D^{1-2\gamma}}{\qty(\mathbb{E}[\epsilon^2]+D^{1-\gamma}+D^{-\gamma})^2}\,.
\end{equation}
In agreement with the result for the mean of the $\GEC$ in \cref{sm:eq:rp:GEC:mean}, we find a qualitative change at $\gamma=1$ going from a vanishing variance $\lim_{D\to\infty}\var[\GEC]_{\gamma<1}=0$ in the ergodic regime to a constant variance $\lim_{D\to\infty}\var[\GEC]_{\gamma>1}=\frac{\var[\epsilon_i^2]}{\mathbb{E}[\epsilon^2]^2}$ in both the fractal and the fully nonergodic phase.
For $\gamma>1$, the corrections to the variance of the $\GEC$ take the form
\begin{equation}\label{sm:eq:rp:GEC:var:fractal}
    \var[\GEC]_{\gamma>1}=\frac{\var[\epsilon_i^2]}{\mathbb{E}[\epsilon^2]^2}
    -\frac{2\var[\epsilon_i^2]}{\mathbb{E}[\epsilon^2]^3}D^{1-\gamma}
    +
    f_1(\gamma,D)\,,
\end{equation}
where $f_1(\gamma,D)$ denotes the subleading corrections.
These change at the ergodicity breaking transition from $f_1(1<\gamma<2,D)=O(D^{2-2\gamma})$ to $f_1(\gamma>2,D)=O(D^{-\gamma})$.

The leading terms in the variance of the $\GEC$ for $\gamma<1$ show an additional change in scaling at $\gamma=\frac{1}{2}$.
Specifically, the leading terms in the ergodic regime are
\begin{equation}
    \var[\GEC]_{\gamma<1/2} \simeq \frac{8}{D}% + O(D^{2-2\gamma})
    \quad \mathrm{and}\quad
    \var[\GEC]_{1/2<\gamma<1} \simeq \frac{\var[\epsilon_i^2]}{D^{2-2\gamma}}\,,
\end{equation}
while at $\gamma=\frac{1}{2}$, they contribute equally as
\begin{equation}
    \var[\GEC]_{\gamma=1/2} \simeq \frac{8+\var[\epsilon_i^2]}{D^{2-2\gamma}}
     = \frac{8+\var[\epsilon_i^2]}{D}\,.
\end{equation}
In contrast to the subleading corrections to the mean in \cref{sm:eq:rp:GEC:mean:ergodic}, here the leading term determines the change of behavior.
This distinction suggests that full GOE behavior is observed for the RPM below $\gamma<\frac{1}{2}$, while in the regime $\frac{1}{2}<\gamma<1$, the RPM admits GOE statistics with non-universal corrections.
Taking into account the next order determines a change of subleading terms from $O(D^{-1})$ for $\frac{1}{2}<\gamma\leq\frac{2}{3}$ to $O(D^{3\gamma-3})$ for $\frac{2}{3}<\gamma<1$.
Finally, at $\gamma=1$ we identify the leading terms of the form
\begin{equation}\label{sm:eq:rp:GEC:var:ergodic}
    \var[\GEC]_{\gamma=1} = \frac{\var[\epsilon_i^2]}{\qty(1+\mathbb{E}[\epsilon])^2}
    +
    \qty[
    \frac{8}{1+\mathbb{E}[\epsilon]}
    +
    \frac{\var[\epsilon_i^2]}{\qty(1+\mathbb{E}[\epsilon])^3}
    ]\frac{1}{D}+O(D^{-2})\,,
\end{equation}
which for a standard Gaussian distribution of $\epsilon_i$ yields $\var[\GEC]_{\gamma=1} = \frac{1}{2} - \frac{15}{4D}+O(D^{-2})$.

\section{\texorpdfstring{Derivation of the $\GEC$ for the QSM model}{Derivation of the GEC for the QSM model}}
Let us proceed with the moments of the $\GEC$ for the QSM.
For ease of reference, let us repeat the definition of the QSM.
The Hamiltonian of the QSM is~\cite{Suntajs2022}
\begin{equation}\label{sm:eq:qsun}
    \qmoperator H_\mathrm{QS} = \qmoperator R + g_0 \sum_{\ell=1}^L \alpha^{u_\ell} \qmoperator S^x_{k(\ell)} \qmoperator S^x_{\ell} + \sum_{\ell=1}^L h_\ell \qmoperator S^z_\ell\,,
\end{equation}
where the random grain is modeled by a normalized GOE matrix $\qmoperator R = \qmoperator M/\sqrt{2^N+1}$.
The random fields, acting on the spins outside the thermal bubble, are uniformly distributed as $h_\ell\in[h-W,h+W]$.
The positions of the outside spins in the exponentially decaying interaction strength $\alpha^{u_\ell}$ is given as $u_\ell=\ell-1+\zeta_\ell$, including a small fluctuation $\zeta_\ell\in[-\zeta,\zeta]$, except to the first coupling, where $u_1=0$.
The model features ETH behavior for $\alpha\gtrsim1$ (see the End matter) and a nonergodic phase at $\alpha<\alpha_c=1/\sqrt{2}$~\cite{DeRoeck2017,DeRoeck2025}.
Recent works show that in the intermediate regime $\alpha_c<\alpha\lesssim1$, the QSM admits a fading ergodicity phase characterized by exponentially slow relaxation~\cite{Kliczkowski2024,Swietek2025a,Swietek2024}.
In this regime, the model obeys RMT behaviour, however, the model thermalizes on exponentially large timescales, which are smaller than the Heisenberg time.

The Hilbert space of the QSM can be decomposed into the degrees of freedom of the thermal grain and the localized spins $\mathcal{H}=\mathcal{H}_\mathrm{grain}\otimes\mathcal{H}_\mathrm{loc}$.
Hence, any product state in the full Hilbert space can be viewed as a tensor product of the associated subspaces $\ket{i}=\ket{n}\otimes\ket{\mu}$, where $\ket{n}\in\mathcal{H}_\mathrm{grain}$ and $\ket{\mu}\in\mathcal{H}_\mathrm{loc}$.
With this decomposition we can express the terms of the $\GEC$ as
\begin{align}
    H_{ii}^2 &= 
    R_{nn}^2 + 2R_{nn}\sum_\ell h_\ell\mel{\mu}{\qmoperator S^z_\ell}{\mu}
    +\sum_{\ell,\ell'}h_\ell h_{\ell'}\mel{\mu}{\qmoperator S^z_\ell \qmoperator S^z_{\ell'}}{\mu}\,,\\
    (\qmoperator H^2)_{ii} &= 
    (\qmoperator R^2)_{nn} + \frac{g_0^2}{16}\sum_{\ell}\alpha^{2u_\ell}
    +\sum_{\ell,\ell'}h_\ell h_{\ell'}\mel{\mu}{\qmoperator S^z_\ell \qmoperator S^z_{\ell'}}{\mu} + 2R_{nn}\sum_\ell h_\ell\mel{\mu}{\qmoperator S^z_\ell}{\mu}\label{sm:eq:qsun:H2ii}\,.
\end{align}
In the second equation we use the fact that the interaction term in $\qmoperator H^2$ only contributes when spin-flips cancel each other, leaving the state invariant, i.e.,~only the term $\ell=\ell'$ survives.
Moreover, the mixed terms containing only a single spin-flip process vanish as they do not have a diagonal part.
Therefore, the numerator of the $\GEC$ is
\begin{equation}\label{sm:eq:qsun:x_i}
    x_i = 2(\qmoperator R^2)_{nn} - R_{nn}^2 
    + \frac{g_0^2}{8}\sum_{\ell}\alpha^{2u_\ell}
    + \sum_{\ell,\ell'}h_\ell h_{\ell'}\mel{\mu}{\qmoperator S^z_\ell \qmoperator S^z_{\ell'}}{\mu} 
    + 2R_{nn}\sum_\ell h_\ell\mel{\mu}{\qmoperator S^z_\ell}{\mu}\,.
\end{equation}
We note that the Hamiltonian in \cref{sm:eq:qsun} is not exactly traceless due to the small size of the random grain.
However, on average, the contribution from the trace vanishes.

\subsection{\texorpdfstring{Mean of the $\GEC$}{Mean of the GEC}}
Since the operator $\qmoperator R$ is a normalized GOE matrix, the variance of its elements is $\overline{R_{nn}^2}=2/(2^N+1)$ and $\overline{R_{nm}^2}=1/(2^N+1)$. 
Thus, the average of the first term evaluates to $\mathbb{E}[2(R^2)_{nn} - R_{nn}^2] = 2^{N+1}/(2^N+1)$.
In the next term, $u_\ell$ is a uniform random variable, hence we can compute the average (and any higher moments) of $\alpha^{ku_\ell}$, resulting in ($\forall \ell>1$)
\begin{equation}\label{sm:eq:qsun:u_l:moments}
    \overline{\alpha^{ku_\ell}} = \int_{\ell-1-\zeta}^{\ell-1+\zeta}\frac{dx}{2\zeta} \alpha^{kx}
    = \frac{\alpha^{k\zeta}-\alpha^{-k\zeta}}{2k\zeta\ln(\alpha)}\alpha^{k(\ell-1)}
    = \frac{\sinh(k\zeta\ln(\alpha))}{k\zeta\ln(\alpha)}\alpha^{k(\ell-1)}
    \equiv F(k\zeta,\alpha)\alpha^{k(\ell-1)}\,.
\end{equation}
Here, we define the function $F(k\zeta,\alpha)=\mathrm{sinhc}(k\zeta\ln(\alpha))$, which has the limiting value $\lim_{\zeta\to0}F(k\zeta,\alpha)=1$.
Then, the sum over $\ell$ can be trivially computed using the properties of a geometric series with ratio $\alpha^2$ (we also need to exclude $u_1=0$ from the average):
\begin{equation}
    \begin{split}
    \sum_{\ell=1}^L\overline{\alpha^{2u_\ell}}
    &= 1 + \sum_{\ell=2}^L\overline{\alpha^{2u_\ell}}
    = 1 + F(2\zeta,\alpha)\sum_{\ell=2}^L \alpha^{2\ell-2} \\
    &= 1 + F(2\zeta,\alpha)\sum_{\ell'=1}^{L-1} \qty(\alpha^2)^{\ell'}
    = 1+F(2\zeta,\alpha)\qty(\frac{1-\alpha^{2L}}{1-\alpha^2}-1)\,.
    \end{split}
\end{equation}
The next term in \cref{sm:eq:qsun:x_i} can be evaluated by noticing that $(1/D)\Tr(\qmoperator S^z_\ell \qmoperator S^z_{\ell'})=\frac{1}{4}\delta_{\ell\ell'}$, while the last term vanishes since $\Tr(\qmoperator S^z_\ell)=0$.
Collecting all the terms leads to the average of the numerator
\begin{equation}
    \mathbb{E}[x] = \frac{2^{N+1}}{2^N+1} + \frac{g_0^2}{8}\qty[1+F(2\zeta,\alpha)\qty(\frac{1-\alpha^{2L}}{1-\alpha^2}-1)]+\frac{L}{4}\qty(h^2+\frac{1}{3}W^2)\,,
\end{equation}
where we used the results known for a uniform distribution $\overline{h_\ell^2}=h^2+\frac{1}{3}W^2$,
and the mean value of the $\GEC$
\begin{equation}\label{sm:eq:qsun:GEC:mean}
    \mathbb{E}[\GEC] = \frac{\frac{2^{N+1}}{2^N+1} + \frac{g_0^2}{8}\qty[1+F(2\zeta,\alpha)\qty(\frac{1-\alpha^{2L}}{1-\alpha^2}-1)]+\frac{L}{4}\qty(h^2+\frac{1}{3}W^2)}{1 + \frac{g_0^2}{16}\qty[1+F(2\zeta,\alpha)\qty(\frac{1-\alpha^{2L}}{1-\alpha^2}-1)]+\frac{L}{4}\qty(h^2+\frac{1}{3}W^2)}\,.
\end{equation}
The calculation of the denominator is analogous to the above when only considering the terms in \cref{sm:eq:qsun:H2ii}.
In this work, we consider only small fluctuations in the position of the outside spins ($\zeta\ll1$), which allows us to approximate $F(k\zeta,\alpha)\approx1$.
While $F(k\zeta, \alpha)$ can be calculated exactly, as above, it is instructive to use this approximation to simplify \cref{sm:eq:qsun:GEC:mean}.
In effect, for the discussed systems, where we consider $\zeta = 0.2$, this approximation is highly accurate, with an error of $|1-F(2\zeta,\alpha)|<5\cdot 10^{-3}$ in the considered range of $\alpha$.
This yields the slightly simpler result for the mean of the $\GEC$
\begin{equation}\label{sm:eq:qsun:GEC:mean2}
    \mathbb{E}[\GEC] \approx \frac{\frac{2^{N+1}}{2^N+1} + \frac{g_0^2}{8}\frac{1-\alpha^{2L}}{1-\alpha^2}+\frac{L}{4}\qty(h^2+\frac{1}{3}W^2)}{1 + \frac{g_0^2}{16}\frac{1-\alpha^{2L}}{1-\alpha^2}+\frac{L}{4}\qty(h^2+\frac{1}{3}W^2)}
    \equiv
    \mathbb{E}[\GEC]^*
    \,,
\end{equation}
where we define $\mathbb{E}[\GEC]^*$ as the average value of the $\GEC$ under the approximation $\zeta\ll1$.
Later, this approximation will become important when deriving a simplified expression for the variance of the $\GEC$.

Similarly as for the RPM, we find that in the (expected) ETH phase ($\alpha\ge 1$, see the discussion in the End Matter), the mean of the $\GEC$ is $\lim_{L\to\infty}\mathbb{E}[\GEC]_{\alpha>1}=2$, while in the fading ergodicity and localized phase ($\alpha<1$) the mean becomes $\lim_{L\to\infty}\mathbb{E}[\GEC]_{\alpha<1}=1$.
The leading corrections, however, differ strongly from the RPM. 
For $\alpha<1$, the leading term is polynomial in the system size as
\begin{equation}\label{sm:eq:qsun:GEC:mean:weak_erg}
    \mathbb{E}[\GEC]^*_{\alpha<1} = 1 + \frac{\frac{g_0^2}{1-\alpha^2}+16\frac{2^N-1}{2^N+1}}{4h^2+\frac{4}{3}W^2}\frac{1}{L}+O\qty(\frac{1}{L^2})\,,
\end{equation}
while in the ergodic phase, the first correction becomes exponentially small in $L$:
\begin{equation}\label{sm:eq:qsun:GEC:mean:ergodic}
    \mathbb{E}[\GEC]^*_{\alpha>1} \approx 2 - \frac{4\qty(h^2+\frac{W^2}{3})}{g_0^2}(\alpha^2-1)\frac{L}{\alpha^{2L}}\,.
\end{equation}
Moreover, at $\alpha=1$, the mean of the $\GEC$ is
\begin{equation}
    \mathbb{E}[\GEC]^*_{\alpha=1} = 1 + \frac{g_0^2}{g_0^2 + 4h^2+\frac{W^2}{3}} + O\qty(\frac{1}{L})\,.
\end{equation}
Therefore, in contrast to the RPM, the corrections to the QSM for $\alpha\leq1$ are polynomial in system size, which we attribute to the quasilocality of the model (the number of nonzero off-diagonal matrix elements is polynomial for the QSM, while it is exponential for the RPM).

\Cref{sm:fig:qsun:mean} shows the comparison of results from ED for small system sizes using \cref{sm:eq:gec:approx:moments} to the analytical expression from \cref{sm:eq:qsun:GEC:mean2}.
We compute the moments of the $\GEC$ numerically using exact diagonalization (ED).
For each realization of the ensemble, we evaluate the mean and variance of $x_i$, as well as the mean of $\sigma^2$.
These quantities are then averaged independently over the ensemble of Hamiltonians.
Finally, we use these ensemble-averaged values to obtain the moments of the $\GEC$ according to \cref{sm:eq:gec:approx:moments}.
We find good agreement of the numerical data and the analytical prediction, suggesting that corrections beyond \cref{sm:eq:qsun:GEC:mean2} are
small.
The mean of the $\GEC$ approaches the thermodynamic-limit result with exponential corrections on the ergodic side [see \cref{sm:eq:qsun:GEC:mean:ergodic}], while in both the fading ergodicity and nonergodic phase, the corrections are polynomial as expected from \cref{sm:eq:qsun:GEC:mean:weak_erg}.

\begin{figure}[t]
    \centering
    \includegraphics[width=0.7\columnwidth]{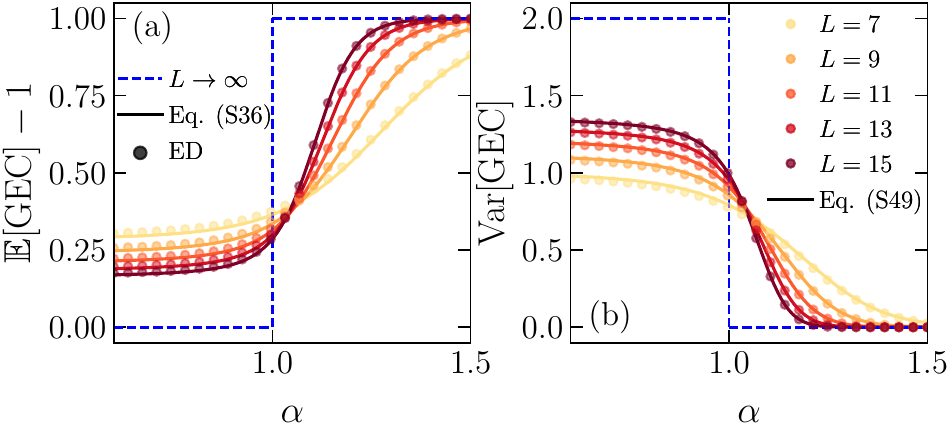}
    {\phantomsubcaption\label{sm:fig:qsun:mean}}
    {\phantomsubcaption\label{sm:fig:qsun:var}}
    \caption{
    Comparison of the \subref{sm:fig:qsun:mean} average mean and \subref{sm:fig:qsun:var} variance of the $\GEC$ for the QSM for different values of $\alpha$ and system sizes $L$ to the analytical predictions of $\mathbb{E}[\GEC]^*$ and $\var[\GEC]^*$ in \cref{sm:eq:qsun:GEC:mean2,sm:eq:qsun:GEC:var}, respectively.
    We choose the following model parameters $N=3$, $g_0=1$, $\zeta=0.2$, $h=1$ and $W=0.5$.
    The data points show results from ED, using the averaging strategy from Eq.~\eqref{sm:eq:gec:approx:moments}, averaged over $N_{\rm dis}=50000$ realizations, while the solid lines are the analytical predictions from\cref{sm:eq:qsun:GEC:mean2,sm:eq:qsun:GEC:var} for the mean and the variance of the $\GEC$, respectively.
    The horizontal dotted lines show the prediction for both quantities for $\alpha=1$, while the dashed line shows the analytical predictions in the thermodynamic limit $L\to\infty$, see the text for details.
    }
    \label{sm:fig:qsun}
\end{figure}

\subsection{\texorpdfstring{Variance of the $\GEC$}{Variance of the GEC}}
Lastly, let us turn to the calculation of the variance of the $\GEC$ for the QSM.
The square of $x_i$ can be expressed as

\begin{equation}\label{sm:eq:qsun:x_i2}
    \begin{split}
        x_i^2 
        &= A_{nn}^2 + \frac{g_0^4}{64}\sum_{\ell,\ell'}\alpha^{2u_\ell}\alpha^{2u_{\ell'}}
        + \sum_{\ell_1,\ell_2,\ell_3,\ell_4} h_{\ell_1}h_{\ell_2}h_{\ell_3}h_{\ell_4}\mel{\mu}{\qmoperator S^z_{\ell_1}\qmoperator S^z_{\ell_2}\qmoperator S^z_{\ell_3}\qmoperator S^z_{\ell_4}}{\mu}\\
        &\qquad
        + \qty[4R_{nn}^2 + 2A_{nn} + \frac{g_0^2}{4}\sum_{\ell}\alpha^{2u_\ell}]\sum_{\ell,\ell'}h_\ell h_{\ell'}\mel{\mu}{\qmoperator S^z_{\ell}\qmoperator S^z_{\ell'}}{\mu}\\
        &\qquad
        +\frac{g_0^2}{4}A_{nn}\sum_{\ell}\alpha^{2u_\ell}
        +2A_{nn}R_{nn}\sum_\ell h_\ell\mel{\mu}{\qmoperator S^z_\ell}{\mu}
        +\frac{g_0^2}{2}R_{nn}\sum_{\ell}\alpha^{2u_\ell}\sum_{\ell'} h_{\ell'}\mel{\mu}{\qmoperator S^z_{\ell'}}{\mu}\\
        &\qquad
        +4R_{nn}\sum_{\ell_1,\ell_2,\ell_3} h_{\ell_1}h_{\ell_2}h_{\ell_3}\mel{\mu}{\qmoperator S^z_{\ell_1}\qmoperator S^z_{\ell_2}\qmoperator S^z_{\ell_3}}{\mu}\,,
    \end{split}
\end{equation}
where $A_{nn}=2(R^2)_{nn}-R^2_{nn}$.
Since most of the terms present in \cref{sm:eq:qsun:x_i2} have been calculated in the context of the mean of the $\GEC$, we can write (note that the last three terms in \cref{sm:eq:qsun:x_i2} vanish in the average since $\mathbb{E}[R_{nn}]=0$)

\begin{equation}\label{sm:eq:qsun:x_i2:av:-1}
    \begin{split}
        \mathbb{E}[x^2]
        &= \frac{1}{2^N}\sum_n\overline{A_{nn}^2}
        + \frac{g_0^4}{64}\sum_{\ell,\ell'}\overline{\alpha^{2u_\ell}\alpha^{2u_{\ell'}}}
        + \sum_{\ell_1,\ell_2,\ell_3,\ell_4}\overline{h_{\ell_1}h_{\ell_2}h_{\ell_3}h_{\ell_4}}\frac{1}{2^L}\sum_\mu\mel{\mu}{\qmoperator S^z_{\ell_1}\qmoperator S^z_{\ell_2}\qmoperator S^z_{\ell_3}\qmoperator S^z_{\ell_4}}{\mu}\\
        &\qquad
        + \qty[4+\frac{4}{2^N+1}+\frac{g_0^2}{4}\qty[1+F(2\zeta,\alpha)\qty(\frac{1-\alpha^{2L}}{1-\alpha^2}-1)]]\frac{L}{4}\qty(h^2+\frac{W^2}{3})\\
        &\qquad
        +\frac{g_0^2}{4}\frac{2^{N+1}}{2^N+1}\qty[1+F(2\zeta,\alpha)\qty(\frac{1-\alpha^{2L}}{1-\alpha^2}-1)]\,.
    \end{split}
\end{equation}
Let us move to the remaining terms in Eq.~\eqref{sm:eq:qsun:x_i2:av:-1}.

The first term can be rewritten as $\overline{A_{nn}^2} = \overline{(R^2)_{nn}^2}-4\overline{(R^2)_{nn}R_{nn}^2}+\overline{R_{nn}^4}$.
Notably, these averages were already computed for a GOE matrix in Eqs.~\eqref{sm:eq:rp:M2ii2} and~\eqref{sm:eq:rp:M2iiMii2}.
Including the normalization of the matrix $\qmoperator R$ and the fourth moment being $\overline{R_{nn}^4} = 3\overline{R_{nn}^2}^2=12/(2^N+1)^2$, we arrive at the expression
\begin{equation}
    \frac{1}{2^N}\sum_n\overline{A_{nn}^2} = \frac{2^{N+2}\qty(2^N+2)}{\qty(2^N+1)^2}\,.
\end{equation}
The second part can be computed using the properties of a geometric series and the result in \cref{sm:eq:qsun:u_l:moments}, namely we find the simple expression
\begin{equation}
    \begin{split}
        \sum_{\ell,\ell'}\overline{\alpha^{2u_\ell}\alpha^{2u_{\ell'}}} 
        &=
        \sum_{\ell}\overline{\alpha^{4u_\ell}}
        +
        \sum_{\ell\neq\ell'}\overline{\alpha^{2u_\ell}}\,\overline{\alpha^{2u_{\ell'}}}
        =\sum_{\ell}\overline{\alpha^{4u_\ell}} + \qty(\sum_{\ell}\overline{\alpha^{2u_\ell}})^2 - \sum_{\ell}\overline{\alpha^{2u_\ell}}^2\\
        &=
        \qty[F(4\zeta,\alpha)-F^2(2\zeta,\alpha)]\qty(\frac{1-\alpha^{4L}}{1-\alpha^2}-1)
        +
        \qty[1+F(2\zeta,\alpha)\qty(\frac{1-\alpha^{2L}}{1-\alpha^2}-1)]^2\\
        &\approx \qty(\frac{1-\alpha^{2L}}{1-\alpha^4})^2\,,
    \end{split}
\end{equation}
where we used the fact that, for small $\zeta$, $F(2\zeta,\alpha)\approx1$ and $F(4\zeta,\alpha)-F^2(2\zeta,\alpha)\approx0$.
To evaluate the third term, we need to break the sum over the four indices $\ell_1,\ell_2,\ell_3$ and $\ell_4$ into smaller terms.
Specifically, the only non-zero elements arise when all indices are equal or when indices appear in pairs such as $(\ell_1=\ell_2,\ell_3=\ell_4)$, $(\ell_1=\ell_3,\ell_2=\ell_4)$ and $(\ell_1=\ell_4,\ell_2=\ell_3)$.
Thus, the last term is simplified to
\begin{equation}
    \sum_{\ell_1,\ell_2,\ell_3,\ell_4}\mathbb{E}\qty[h_{\ell_1}h_{\ell_2}h_{\ell_3}h_{\ell_4}\mel{\mu}{\qmoperator S^z_{\ell_1}\qmoperator S^z_{\ell_2}\qmoperator S^z_{\ell_3}\qmoperator S^z_{\ell_4}}{\mu}]
    =
    \frac{1}{16}\sum_\ell\mathbb{E}[h_\ell^4]
    +
    \frac{3}{16}\sum_{\ell\neq\ell'}\mathbb{E}[h_\ell^2]\mathbb{E}[h_{\ell'}^2]\,,
\end{equation}
where the factor $3$ arises due to the three distinct ways of pairing the indices.
Using known expressions for expectation values in a uniform distribution, we find
\begin{equation}
    \sum_{\ell_1,\ell_2,\ell_3,\ell_4}\overline{h_{\ell_1}h_{\ell_2}h_{\ell_3}h_{\ell_4}}\frac{1}{2^L}\sum_\mu\mel{\mu}{\qmoperator S^z_{\ell_1}\qmoperator S^z_{\ell_2}\qmoperator S^z_{\ell_3}\qmoperator S^z_{\ell_4}}{\mu}]
    =
    \frac{L}{16}\qty(h^4+2h^2W^2+\frac{W^4}{5})
    +
    \frac{3L(L-1)}{16}\qty(h^2+\frac{W^2}{3})^2\,.
\end{equation}
Collecting all terms we arrive at the second moment of $x_i$

\begin{equation}\label{sm:eq:qsun:x_i2:av}
    \begin{split}
        \mathbb{E}[x^2]^*
        &= \frac{2^{N+2}\qty(2^N+2)}{\qty(2^N+1)^2}
        + \frac{g_0^4}{64}\qty(\frac{1-\alpha^{2L}}{1-\alpha^2})^2\\
        &\qquad
        + \frac{L}{16}\qty(h^4+2h^2W^2+\frac{W^4}{5})
        +
        \frac{3L(L-1)}{16}\qty(h^2+\frac{W^2}{3})^2\\
        &\qquad
        + \qty[\frac{2^{N+2}+8}{2^N+1}+\frac{g_0^2}{4}\qty(\frac{1-\alpha^{2L}}{1-\alpha^2})]\frac{L}{4}\qty(h^2+\frac{W^2}{3})\\
        &\qquad
        +\frac{g_0^2}{4}\frac{2^{N+1}}{2^N+1}\qty(\frac{1-\alpha^{2L}}{1-\alpha^2})\,,
    \end{split}
\end{equation}
where we use again the notation that $\mathbb{E}[x^2]^*$ denotes the average under the approximation when $\zeta\ll1$.
The square of the first moment is
\begin{equation}\label{sm:eq:qsun:x_i:av2}
    \begin{split}
        (\mathbb{E}[x]^*)^2
        &= \frac{2^{2N+2}}{(2^N+1)^2} + \frac{g_0^4}{64}\qty(\frac{1-\alpha^{2L}}{1-\alpha^2})^2
        +\frac{L^2}{16}\qty(h^2 + \frac{W^2}{3})^2\\
        &\qquad
        +\frac{g_0^2}{4}\frac{2^{N+1}}{2^N+1}\frac{1-\alpha^{2L}}{1-\alpha^2}
        +\frac{L}{2}\frac{2^{N+1}}{2^N+1}\qty(h^2 + \frac{W^2}{3})\\
        &\qquad
        +\frac{g_0^2L}{16}\qty(h^2 + \frac{W^2}{3})\frac{1-\alpha^{2L}}{1-\alpha^2}\,,
    \end{split}
\end{equation}
which leads to the variance of $x_i$
\begin{equation}\label{sm:eq:qsun:x_i:var}
    \begin{split}
        \var[x] &\approx \var[x]^* = \mathbb{E}[x^2]^* - (\mathbb{E}[x]^*)^2\\
        &= \frac{2^{N+3}}{(2^N+1)^2} 
        + \frac{L}{16}\qty(h^4+2h^2W^2+\frac{W^4}{5})\\
        &\qquad
        + \frac{2L^2-3L}{16}\qty(h^2+\frac{W^2}{3})^2
        + \frac{L}{2}\frac{4}{2^N+1}\qty(h^2 + \frac{W^2}{3})\,.
    \end{split}
\end{equation}
We finally obtain an expression for the variance of the $\GEC$: 
\begin{equation}\label{sm:eq:qsun:GEC:var}
    \var[\GEC]^* = \frac{\frac{2^{N+3}}{(2^N+1)^2} 
        + \frac{L}{16}\qty(h^4+2h^2W^2+\frac{W^4}{5})
        + \frac{2L^2-3L}{16}\qty(h^2+\frac{W^2}{3})^2
        + \frac{2L}{2^N+1}\qty(h^2 + \frac{W^2}{3})}{\qty[1 + \frac{g_0^2}{16}\frac{1-\alpha^{2L}}{1-\alpha^2}+\frac{L}{4}\qty(h^2+\frac{1}{3}W^2)]^2}\,.
\end{equation}
It is remarkable that the $\alpha$-dependence is solely given by the denominator.
It is straightforward to find the leading term for the variance of the $\GEC$ in the expected ETH phase for $\alpha\ge 1$:
\begin{equation}\label{sm:eq:qsun:GEC:var:ergodic}
    \var[\GEC]^*_{\alpha>1} \approx \frac{32\qty(h^2+\frac{W^2}{3})^2}{g_0^4}(\alpha^2-1)^2\frac{L^2}{\alpha^{4L}}\,.
\end{equation}
In the fading ergodicity and nonergodic phase, we obtain the leading terms
\begin{equation}\label{sm:eq:qsun:GEC:var:fading}
    \var[\GEC]^*_{\alpha<1} \approx 2
    -
    \qty[\frac{2\qty(3h^4+\frac{W^4}{5}-\frac{16\qty(3h^2+W^2)}{2^N+1})}{3\qty(h^2+\frac{W^2}{3})^2}
    +
    \frac{16+\frac{g_0^2}{1-\alpha^2}}{h^2+\frac{W^2}{3}}
    ]\frac{1}{L}\,.
\end{equation}
The error of the averaging strategy, where we average the numerator and denominator separately, is of the same order (or slightly larger) than the expressions in \cref{sm:eq:qsun:GEC:var:ergodic,sm:eq:qsun:GEC:var:fading}.
Therefore we do not investigate the subleading terms of $\var[\GEC]^*$.
We note again the strong contrast with exponential corrections $O(\alpha^{-2L})$ on the ergodic side for $\alpha>1$ and polynomial corrections $O(L^{-1})$ for $\alpha<1$.
This distinction hints towards strongly non-universal corrections to the $\GEC$.
Finally, at the wEBT at $\alpha=1$, we find a constant factor with polynomial corrections
\begin{equation}\label{sm:eq:qsun:GEC:var:transition}
    \var[\GEC]^*_{\alpha=1} = \frac{2
    \qty(h^2+\frac{W^2}{3})^2}{\qty(\frac{g_0^2}{4}+h^2+\frac{W^2}{3})^2}
    +
    O\qty(\frac{1}{L})\,.
\end{equation}

In \cref{sm:fig:qsun:var} we compare the numerically computed variance of the $\GEC$ using Eq.~\eqref{sm:eq:gec:approx:moments} to the analytical predicion in Eq.~\eqref{sm:eq:qsun:GEC:var}.
The analytical prediction for the variance of the $\GEC$ works well when considering $\zeta\ll1$.

\section{\texorpdfstring{Estimation of corrections to the variance of the $\GEC$}{Estimation of corrections to the varance of the GEC}}\label{sm:sec:approx:validity}
Before moving on to the TLG model, we discuss the approximation used in the ensemble averaging.
Specifically, we compare the ensemble-averaged variance of the $\GEC$ as defined in Eq.~\eqref{sm:eq:gec:def} to the approximation of performing the average of the numerator and denominator of the $\GEC$ separately in \cref{sm:eq:gec:approx:moments}.
The resulting corrections in the example of the RPM in \cref{sm:fig:rp:err} decay with the matrix dimension as $1/D$ for $\gamma>1$ or faster in the ergodic regime for $\gamma\leq1$.
Therefore, the corrections lie well below the first subleading terms studied in Eqs.~\eqref{sm:eq:rp:GEC:var:fractal}--\eqref{sm:eq:rp:GEC:var:ergodic}.
This allows us to correctly identify the additional change in scaling of the subleading terms at $\gamma=1/2$.
However, the change of subleading corrections at $\gamma=2$ remains an open question since the error on finite systems that stems from the averaging strategy is of the same order as the leading corrections.

In the case of the QSM, the correction due to the averaging strategy becomes more prominent, shown in \cref{sm:fig:qsun:err}.
The leading corrections in Eqs.~\eqref{sm:eq:qsun:GEC:var:ergodic}--\eqref{sm:eq:qsun:GEC:var:transition} show a change from exponential $O(\alpha^{-4L})$ corrections in the ergodic regime to polynomial corrections of the order $O(1/L)$ at $\alpha\leq1$.
While a similar trend is seen in the error due to the averaging strategy from Eq.~\eqref{sm:eq:gec:approx:moments}, the exact rate of the decay differs and might even be sublinear, i.e., larger than $1/L$ for $\alpha<1$.
In the ergodic regime at $\alpha>1$, we again find exponential corrections, which appear to be of the same order as the analytically predicted subleading terms in Eq.~\eqref{sm:eq:qsun:GEC:var:ergodic}.

\begin{figure}[t]
    \centering
    \includegraphics[width=0.7\columnwidth]{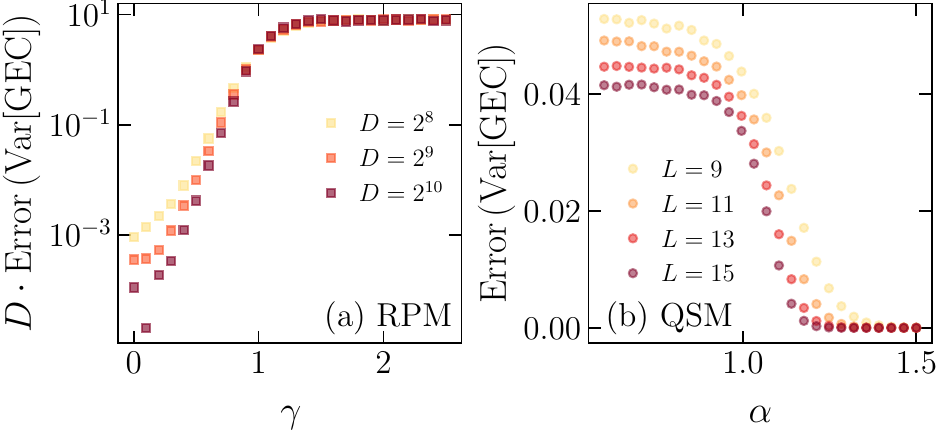}
    {\phantomsubcaption\label{sm:fig:rp:err}}
    {\phantomsubcaption\label{sm:fig:qsun:err}}
    \caption{ Error in the estimate of the variance  for the \subref{sm:fig:rp:err} RPM and \subref{sm:fig:qsun:err} QSM for different values of $\alpha$ and system sizes $L$.
    We plot the absolute value of the difference between the variance calculated exactly following the definition of the $\GEC$ in \cref{sm:eq:gec:def} and the variance obtained from the averaging strategy in \cref{sm:eq:gec:approx:moments}.
    We choose the following model parameters for the QSM: $N=3$, $g_0=1$, $\zeta=0.2$, $h=1$ and $W=0.5$.
    We rescale the error for the RPM in \subref{sm:fig:rp:err} by the matrix dimension $D$ to visualize that the error is $O(1/D)$ for $\gamma\geq1$, while it becomes significantly smaller in the ergodic phase for $\gamma<1$.
    As a result, the leading corrections to the variance of the $\GEC$ in Eqs.~\eqref{sm:eq:rp:GEC:var:fractal}--\eqref{sm:eq:rp:GEC:var:ergodic} can be obtained faithfully.
    In contrast, we find that in the QSM [data shown in \subref{sm:fig:qsun:err}] the error is polynomially small in the fading-ergodicity regime, while it becomes  exponentially small in the ergodic phase.
    The data points show results from ED averaged over $N_{\rm dis}=4000$ realizations for the RPM and $N_{\rm dis}=50000$ for the QSM.
    }
    \label{sm:fig:error}
\end{figure}

\section{\texorpdfstring{Semianalytic evaluation of $\GEC$ for the TLG model}{Semianalytic evaluation of GEC for the TLG model}}
For the calculation of the variance of the $\GEC$ in the TLG model, we employ a semianalytical approach, which allows us to reach system sizes of up to $L=450$, which are inaccessible in ED.
The model is defined via the Hamiltonian
\begin{equation}\label{sm:eq:tlg}
    \qmoperator H_\mathrm{TLG} = \sum_{\langle \ell,\ell' \rangle} \qmoperator C_{\ell\ell'} \big[ 
        -t_0(\qmoperator c_\ell^\dagger \qmoperator c_{\ell'} + \hc)
        + V (\qmoperator n_\ell (\mathbb{1} - \qmoperator n_{\ell'}) + (\mathbb{1} - \qmoperator n_\ell) \qmoperator n_{\ell'})
    \big]\,,
\end{equation}
where $\langle \ell,\ell' \rangle$ denotes 
nearest-neighbor sites on the triangular lattice (see \cref{sm:fig:tlg_sketch}) and ${\qmoperator C_{\ell\ell'} = \mathbb{1} - \prod_{k \in \mathcal{N}(\ell,\ell')}\qmoperator n_k}$ is the kinetic constraint,
while we denote $\mathcal{N}(\ell, \ell')$ as the common neighborhood of sites $\ell$ and $\ell'$ on the triangular ladder.
Specifically, this constraint allows for a particle to hop from site $\ell$ to site $\ell'$ if in the joined neighborhood of both sites, there exist at least one hole (particles are prohibited to move if in the surrounding only the destination site is empty).

We rewrite the Hamiltonian in \cref{sm:eq:tlg} as a sum of diagonal and off-diagonal terms $\qmoperator{H} = -t_0\qmoperator{A} + V\qmoperator{H}_d$, defined respectively as
\begin{align}
    \qmoperator H_d &= \sum_{\langle \ell,\ell' \rangle} \qmoperator C_{\ell\ell'}(\qmoperator n_\ell + \qmoperator n_{\ell'} - 2\qmoperator n_\ell \qmoperator n_{\ell'})
    \\
    \qmoperator A &= \sum_{\langle \ell,\ell' \rangle} \qmoperator C_{\ell\ell'}(\qmoperator c_\ell^\dagger \qmoperator c_{\ell'} + \hc)\,.
\end{align}
Therefore, the only terms entering $\GEC(\ket{i})$ are $\mel{i}{\qmoperator H_d}{i}\equiv (H_d)_{ii}$ and $\mel{i}{\qmoperator A^2}{i}$.
This particular decomposition allows for a simplification of the expression of the $\GEC$ by noticing that $\mel{i}{\qmoperator A^2}{i} = (H_d)_{ii}$ holds true (which can be obtained by finding that the only contributing terms to $\mel{i}{\qmoperator A^2}{i}$ are moving a particle from site $\ell$ to $\ell'$ and back to leave the state invariant) and therefore, $x_i = 2t_0^2(H_d)_{ii} + V^2(H_d)_{ii}^2$.
In the next step, we need to exclude the mean of the Hamiltonian in the $\GEC$, which can simply be found by the substitution $(H_d)_{ii}\to (H_d)_{ii}-\frac{1}{D}\Tr{\qmoperator H}$.
Next, let us define the mean of the diagonal term
\begin{equation}
    \mathbb{E}[H_d] \equiv \frac{1}{D}\sum_i (H_d)_{ii} = \frac{1}{D}\Tr{\qmoperator H}
\end{equation}
and all the higher moments
\begin{equation}
    \mathbb{E}[(H_d)^k] \equiv \frac{1}{D}\sum_i (H_d)_{ii}^k\,,
\end{equation}
such that the width of the Hamiltonian is $\frac{1}{D}\Tr{\qmoperator H^2} = t_0^2\mathbb{E}[H_d] + V^2\mathbb{E}[(H_d)^2] - V^2\mathbb{E}[H_d]^2$.
This allows one to write the mean of the $\GEC$ in terms of the moments $\mathbb{E}[(H_d)^k]$ as
\begin{equation}\label{sm:eq:tlg:mean}
    \mathbb{E}[\GEC] = \frac{2t_0^2\mathbb{E}[H_d] + V^2\mathbb{E}[(H_d)^2] - V^2\mathbb{E}[H_d]^2}{t_0^2\mathbb{E}[H_d] + V^2\mathbb{E}[(H_d)^2] - V^2\mathbb{E}[H_d]^2}\,.
\end{equation}

The second moment of the $\GEC$ can be expressed in a similar fashion as the mean in \cref{sm:eq:tlg:mean} with
\begin{equation}
    \begin{split}
        \mathbb{E}[\GEC^2] =& \frac{
    4t_0^4\mathbb{E}[(H_d)^2]
    + V^4\qty(\mathbb{E}[(H_d)^4] - 3\mathbb{E}[H_d]^4 + 6\mathbb{E}[(H_d)^2]\,\mathbb{E}[H_d]^2 - 4\mathbb{E}[(H_d)^3]\,\mathbb{E}[H_d])
    }{
    \qty[t_0^2\mathbb{E}[H_d] + V^2\mathbb{E}[(H_d)^2] - V^2\mathbb{E}[H_d]^2]^2}\\
    &+
    \frac{4t_0^2V^2\qty(\mathbb{E}[(H_d)^3] + \mathbb{E}[H_d]^3 - 2\mathbb{E}[H_d]\,\mathbb{E}[(H_d)^2])
    }{
    \qty[t_0^2\mathbb{E}[H_d] + V^2\mathbb{E}[(H_d)^2] - V^2\mathbb{E}[H_d]^2]^2}\,.
    \end{split}
\end{equation}
Hence, the variance of the $\GEC$ is simply $\var[\GEC] = \mathbb{E}[\GEC^2] - \mathbb{E}[\GEC]^2$.
Since we were not able to find an exact analytical expression for the moments of the $\GEC$, in the following, we describe a semianalytical approach to reach  large system sizes.

\begin{figure}[t]
    \centering
    \includegraphics[width=0.7\columnwidth]{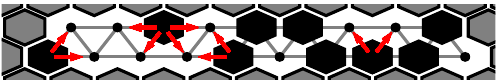}
    \caption{ Sketch of the triangular lattice gas Hamiltonian. The black hexagons denote the particles moving on a triangular lattice, while the red arrows show the allowed movements of the particles due to the kinetic constraint.
    }
    \label{sm:fig:tlg_sketch}
\end{figure}

The cornerstone of the calculation is that any higher-order term $\mathbb{E}[(H_d)^k]$ can be computed in $O(L^k)$ time due to the idempotency of the occupation operators $\qmoperator n_\ell$, \ie $\qmoperator n_\ell^k = \qmoperator n_\ell$ for any integer $k\geq1$.
A second ingredient is the fact that for a set of mutually distinct indices $\ell_1\neq...\neq\ell_p$, one can evaluate the following trace of a product of density operators in the canonical ensemble
\begin{equation}
    \Tr{\qmoperator n_{\ell_1}\cdots\qmoperator n_{\ell_p}}_{\rm C} = \frac{N(N-1)\cdots(N-p+1)}{L(L-1)\cdots(L-p+1)}\,,
\end{equation}
where $N$ is the number of particles in the lattice and $n=N/L$ is the particle filling, or in the grand-canonical ensemble
\begin{equation}
    \Tr{\qmoperator n_{\ell_1}\cdots\qmoperator n_{\ell_p}}_{\rm GC} = n^p\,.
\end{equation}
Therefore, the problem of evaluating $\mathbb{E}[(H_d)^k]$ reduces to adding coefficients in front of the terms $\qmoperator n_{\ell_1}\cdots\qmoperator n_{\ell_p}$ of different length $1\leq p\leq 4k$.
We developed an efficient code to evaluate all higher order terms up to $k=4$ in order to evaluate the mean $\mathbb{E}[\GEC]$ and the variance $\var[\GEC]$ of the $\GEC$.

\bibliography{references.bib}
\end{document}
